# Supplementary material for: Yet anOther Dose Algorithm (YODA) for independent computations of dose and dose changes due to anatomical changes
Source: arXiv:2404.00976 source file (2024-04-01)
Supplement: Supplementary file 1 [file appendix.tex]

\section{Appendix}
The Gateaux-differential of $E_{D_k}$ is given by
\begin{align*}
    \var{E_{D_k}(\vb{e^0}, \vb{h})}
     & = \int\limits_{D_k} \dd V \frac{h_{\rho_k}(\vb{r}) \rho_c(z) - \rho_k(\vb{r}) h_{\rho_c}(z)}{\rho_c^2(z)} \Psi_{FE}(\vb{r}, \vb{e^0}) D_{FP}(z, \vb{e^0}) \tag{direct effect} \\
     & + \int\limits_{D_l} \dd V \frac{\rho_k(\vb{r})}{\rho_c(z)} \var{\Psi_{FE}(\vb{r}, \vb{e^0}, \vb{h})} D_{FP}(z, \vb{e^0}) \label{eq:var_R_FE} \tag{direct and indirect effect} \\
     & + \int\limits_{D_l} \dd V \frac{\rho_k(\vb{r})}{\rho_c(z)} \Psi_{FE}(\vb{r}, \vb{e^0}) \var{D_{FP}(z, \vb{e^0}, \vb{h})}. \tag{direct and indirect effect}                    \\
     & = \var{R_{l1}(\vb{e^0}, \vb{h})} + \var{R_{l2}(\vb{e^0}, \vb{h})} + \var{R_{l3}(\vb{e^0}, \vb{h})}
\end{align*}
The first contribution to the \textbf{direct effect} is found to be
\begin{equation*}
    \var{R(\vb{e^0}, \vb{h})}_{d} \mathrel{+}= \mathlarger{\displaystyle\sum\limits_{k}} \int\limits_{D_k} \dd V \frac{h_{\rho_k}(\vb{r}) \rho_c(z) - \rho_k(\vb{r}) h_{\rho_c}(z)}{\rho_c^2(z)} \Psi_{FE}(\vb{r}, \vb{e^0}) D_{FP}(z, \vb{e^0})
\end{equation*}
The integrals $\var{R_{l2}(\vb{e^0}, \vb{h})}$ and $\var{R_{l3}(\vb{e^0}, \vb{h})}$ must be worked further to separate the indirect effect from the direct one. Thus, the Gateaux-differential of $\Psi_{FE}(\vb{r}, \vb{e^0})$ in $\var{R_{l2}(\vb{e^0}, \vb{h})}$ is found to be
\begin{align*}
    \var{\Psi_{FE}(\vb{r}, \vb{e^0}, \vb{h})}
     & =
    \Psi_{FE}(\vb{r}, \vb{e^0}) \frac{2 h_{A_{FE}}}{A} \tag{direct effect, ignored}                                                                                                                                           \\
     & + \Psi_{FE}(\vb{r}, \vb{e^0}) \var{\xi}(z, \vb{e^0}, \vb{h}) \underbrace{\qty[\frac{-1}{\xi(z, \vb{e^0})} + \frac{x^2 + y^2}{2} \frac{1}{\xi^2(z, \vb{e^0})} ]}_{P(\vb{r}, \vb{e^0})} \tag{direct and indirect effect}
\end{align*}
Ignoring perturbations in the initial condition of the FE flux (i.e. perturbations in the spot size, spot angular divergence and spot correlation), the Gateaux-differential of the spatial variance of the FE flux is given by
\begin{align*}
    \var{\xi}(z, \vb{e^0}, \vb{h}) = \int\limits_0^z \dd z' (z-z')^2 \var{\overline{\Sigma_{tr}}}(z', \vb{e^0}, \vb{h})
\end{align*}
The energy-flux averaged transport cross section is given by
\begin{align*}
    \overline{\Sigma_{tr}}(z, \vb{e^0})
     & = \frac{1}{N_p(z)} \int \dd E \varphi_{FP}(z, E) \Sigma_{tr}(z, E)
\end{align*}
where
\begin{equation*}
    N_p(z, \varphi_{FP}) = \int \dd E \varphi_{FP}(z, E).
\end{equation*}
The Gateaux-differential of $\overline{\Sigma_{tr}}(z, \vb{e^0})$ is found to be
\begin{align*}
    \var{\overline{\Sigma_{tr}}}(z, \vb{e^0}, \vb{h})
     & = \int \dd E h_\varphi(z, E) \frac{N_p(z) \Sigma_{tr}(z,E) - \Sigma_\varphi(z)}{N_p(z)^2} \tag{indirect effect} \\
     & + \int \dd E \varphi_{FP}(z, E) \frac{h_{\Sigma_{tr}}(z, E)}{N_p(z)} \tag{direct effect}
\end{align*}
where
\begin{equation*}
    \Sigma_\varphi(z, \vb{e^0}) = \int \dd E \varphi_{FP}(z, E) \Sigma_{tr}(z, E).
\end{equation*}
Introducing this back into $\var{\xi}(z, \vb{e^0}, \vb{h})$ gives
\begin{align*}
    \var{\xi}(z, \vb{e^0}, \vb{h})
     & = \int\limits_0^z \dd z' (z-z')^2 \int \dd E h_\varphi(z', E) \frac{N_p(z') \Sigma_{tr}(z',E) - \Sigma_\varphi(z')}{N_p(z')^2} \tag{indirect effect} \\
     & +  \int\limits_0^z \dd z' (z-z')^2 \int \dd E \varphi_{FP}(z', E) \frac{h_{\Sigma_{tr}}(z', E)}{N_p(z')} \tag{direct effect}
\end{align*}
The indirect effect is re-written s.t. the integral over $z'$ covers the semi-infinite region of $(0,\infty)$, namely
\begin{align*}
    \var{\xi}(z, \vb{e^0}, \vb{h})_i = \int\limits_0^\infty \dd z' \int \dd E h_\varphi(z', E) H(z-z') (z-z')^2 \frac{N_p(z') \Sigma_{tr}(z',E) - \Sigma_\varphi(z')}{N_p(z')^2}.
\end{align*}
As already mentinoed, we ignore the perturbation in the initial condition of the Fermi-Eyges solution (i.e. $h_{A_{FE}} = 0$). This perturbation leads only to a direct effect and can model perturbations in the particle numbers or the more clinically relevant delivered MU values. Thus, the \textbf{direct effect} from the $\var{R_{l2}(\vb{e^0}, \vb{h})}$ is
\begin{align*}
    \mathlarger{\displaystyle\sum\limits_{k}} \int\limits_{D_k} \dd V \frac{\rho_k(\vb{r})}{\rho_c(z)} D_{FP}(z, \vb{e^0}) \Psi_{FE}(\vb{r}, \vb{e^0}) P(\vb{r}, \vb{e^0}) \int\limits_0^z \dd z' (z-z')^2 \int \dd E \varphi_{FP}(z', E) \frac{h_{\Sigma_{tr}}(z', E)}{N_p(z')}
\end{align*}
The \textbf{indirect effect} from $\var{R_{l2}(\vb{e^0}, \vb{h})}$ is
\begin{align*}
     & \mathlarger{\displaystyle\sum\limits_{k}} \int\limits_{D_k} \dd V \frac{\rho_k(\vb{r})}{\rho_c(z)} D_{FP}(z, \vb{e^0}) \Psi_{FE}(\vb{r}, \vb{e^0}) P(\vb{r}, \vb{e^0}) \int\limits_0^\infty \dd z' \int \dd E h_\varphi(z', E) H(z-z') (z-z')^2 \frac{N_p(z') \Sigma_{tr}(z',E) - \Sigma_\varphi(z')}{N_p(z')^2} \\
     & =
    \int\limits_0^\infty \dd z' \int \dd E h_\varphi(z', E) \frac{N_p(z') \Sigma_{tr}(z',E) - \Sigma_\varphi(z')}{N_p(z')^2} \mathlarger{\displaystyle\sum\limits_{k}} \int\limits_{D_k} \dd V \frac{\rho_k(\vb{r})}{\rho_c(z)} D_{FP}(z, \vb{e^0}) \Psi_{FE}(\vb{r}, \vb{e^0}) P(\vb{r}, \vb{e^0}) H(z-z') (z-z')^2    \\
     & =
    \langle h_\varphi(z', E), r^\dagger_2(z', E) \rangle
\end{align*}
where the source contribution of the indirect effect has been denoted by $r^\dagger_2(z', E)$.

The equation for $D_{FP}(z, \vb{e^0})$ is repeated here for convenience
\begin{align*}
    D_{FP}(z, \vb{e^0}) & = E S \varphi_{FP}\eval{}_{E_{-}} + \sum\limits_{\Gamma_i} - \qty[\varphi] T + \int\limits_{E_{-}}^{E_{+}} \dd E \qty(S \varphi_{FP} + T \pdv{\varphi_{FP}}{E} + E \Sigma_a \varphi_{FP}) \\
                        & = \int\limits_{E_{-}}^{E_{+}} \dd E \varphi_{FP} \qty[
        E S \delta(E - E_{-}) + S - T \delta(E - E_{-}) -  \dv{T}{E}
        + \qty(\sum\limits_{\Gamma_i}
        \qty(- \delta(E - E_i^-) + \delta(E - E_i^+)) T(E_i))
        + E \Sigma_a
    ]
\end{align*}
The Gateaux-differential of this is given as
\begin{align*}
     & \var{D_{FP}(z, \vb{e^0}, \vb{h})}                          \\
     & = \int\limits_{E_{-}}^{E_{+}} \dd E h_{\varphi_{FP}} \qty[
        E S \delta(E - E_{-}) + S - T \delta(E - E_{-}) -  \dv{T}{E}
        + \qty(\sum\limits_{\Gamma_i}
        \qty(- \delta(E - E_i^-) + \delta(E - E_i^+)) T(E_i))
        + E \Sigma_a
    ] \tag{indirect effect}                                       \\
     & + \int\limits_{E_{-}}^{E_{+}} \dd E \varphi_{FP} \qty[
        E h_S \delta(E - E_{-}) + h_S - h_T \delta(E - E_{-}) -  \dv{h_T}{E}
        + \qty(\sum\limits_{\Gamma_i}
        \qty(- \delta(E - E_i^-) + \delta(E - E_i^+)) h_T(E_i))
        + E h_{\Sigma_a}
    ]
    \tag{direct effect}
\end{align*}
The \textbf{direct effect} from $\var{D_{FP}(z, \vb{e^0}, \vb{h})}$ is found to be
\begin{align*}
     & \mathlarger{\displaystyle\sum\limits_{k}} \int\limits_{D_k} \dd V \frac{\rho_k(\vb{r})}{\rho_c(z)} \Psi_{FE}(\vb{r}, \vb{e^0})                                                                                                       \\
     & \cdot \int\limits_{E_{-}}^{E_{+}} \dd E \varphi_{FP} \qty[E h_S \delta(E - E_{-}) + h_S - h_T \delta(E - E_{-}) -  \dv{h_T}{E}+ \qty(\sum\limits_{\Gamma_i} \qty(- \delta(E - E_i^-) + \delta(E - E_i^+)) h_T(E_i)) + E h_{\Sigma_a}
    ]
\end{align*}
The \textbf{indirect effect} from $\var{D_{FP}(z, \vb{e^0}, \vb{h})}$ is found to be
\begin{align*}
     & \mathlarger{\displaystyle\sum\limits_{k}} \int\limits_{D_k} \dd V \frac{\rho_k(\vb{r})}{\rho_c(z)} \Psi_{FE}(\vb{r}, \vb{e^0}) \\
     & \cdot  \int\limits_{E_{-}}^{E_{+}} \dd E h_{\varphi_{FP}} \qty[
        E S \delta(E - E_{-}) + S - T \delta(E - E_{-}) -  \dv{T}{E}
        + \qty(\sum\limits_{\Gamma_i}
        \qty(- \delta(E - E_i^-) + \delta(E - E_i^+)) T(E_i))
        + E \Sigma_a
    ]
\end{align*}
To write this as an inner-product the domain $D_k$ is split s.t.
\begin{equation*}
    \int\limits_{D_k} \dd V = \int\limits_{z_-}^{z^+} \dd z \iint\limits_{D_{k, xy(z)}} \dd x \dd y.
\end{equation*}
Using this, the \textbf{indirect effect} is re-written as
\begin{align*}
    \int \dd E \int \dd z h_{\varphi_{FP}} & \qty[ E S \delta(E - E_{-}) + S - T \delta(E - E_{-}) -  \dv{T}{E} + \qty(\sum\limits_{\Gamma_i} \qty(- \delta(E - E_i^-) + \delta(E - E_i^+)) T(E_i)) + E \Sigma_a]                     \\
                                           & \cdot \mathlarger{\displaystyle\sum\limits_{k}} \int\limits_{D_k} \dd V \frac{\rho_k(\vb{r})}{\rho_c(z)} \Psi_{FE}(\vb{r}, \vb{e^0})= \langle h_\varphi(z, E), r^\dagger_1(z, E) \rangle
\end{align*}

In the case when the response is the dose, the term $\rho_k(\vb{r})$ is ignored from all of the above equations and the term $\rho_c(z)$ is replaced by $\Delta v \rho_c(z)$.
\end{document}
